# Supplementary material for: Honesty is the Best Policy: On the Accuracy of Apple Privacy Labels Compared to Apps' Privacy Policies
Source: arXiv:2306.17063 source file (2024-06-16)
Supplement: Supplementary file 1 [file additional-data-practices.tex]

\section{Data Practices Beyond Privacy Labels}
\label{sec:additional-data-practices}

%Apple's privacy labels are designed to inform users about an app's data collection practices. However, 
Privacy policies also cover other privacy-relevant data practices that are not options in the labels. In this section, we highlight a few of these practices and provide insight into additional information that can benefit users but is missing from the privacy labels.

\childrenRatingsCountByPrivacyLabel

\adam{I might argue that we drop this section and move the child apps below into the prior results section. I'm not sure how much this is adding. We do have the space.}

\paragraph{Apps Targeting Children.} 
%Apple does not provide a way for developers to indicate differences in their data collection practices based on app features and audiences. It instead informs users about the potential for such variations in a note below the privacy labels for each app, \textit{``Privacy practices may vary, for example, based on the features you use or your age.''}
%
Developers provide a \textit{Content Rating} as part of the app metadata to indicate the age appropriateness of their apps. These ratings are reviewed by Apple~\cite{Apple:Guidelines}, and used to enforce parental control features that restrict children from accessing the app. 
We find that most apps that we analyzed had a 4+ content rating on the App Store (75.98\%; $n=419,762$), while fewer apps had 9+ (0.3\%; $n=16,687$), 12+ (0.8\%; $n=46,737$), or 17+ (1.3\%; $n=69,309$) content rating values. Since privacy labels do not indicate the app's data practices specific to children, the only other option that users have for learning this information is to review the  privacy policy. Given parental control settings, an app with a 4+, 9+, or 12+ rating could be used by minors, although this may not be intended audience for the app. But when an app specifically targets children, it is subject to additional regulation that may require parental consent.
%
%While privacy labels do not specifically describe data practices surrounding children, 
Polisis can identify policy segments that address \textit{International/Specific Audiences} and further identify if the segment addresses \textit{Children}, and then compare this output to the content rating.
%also addresses this audience in their privacy policies.
%
Only 46\% ($n=191,120$) apps with a 4+ content rating also included a privacy policy segment that addresses data practices specific to children. We were more likely to find similar policy segments for apps with different content ratings that can also be accessed by children, 9+ (64\%; $n=10,700$) and 12+ (50\%; $n=23,529$).

We further looked at app content ratings for different privacy label types associated with data collection. These findings are presented in \autoref{fig:children}. Considering apps with a 4+ content ratings, we find that across privacy types, roughly half of these apps had a policy in place that specifically addressed children. While 18\% ($n=75,346$), 37\% ($n=154,972$), and 44\% ($n=184,722$) of the apps with a 4+ content rating declare in their privacy label that they collect data that is used to track users, linked to users, and not linked to user's respectively. Only 53\% ($n=40,081$), 48\% ($n=74,829$), and 49\% ($n=90,755$) of those apps also addressed children in their privacy policies.
Adding a 4+ content rating may help developers reach a wider audience, only  half of these apps consider data practices specific to children in the privacy policy. Our findings are a cause for concern, especially in light  of COPPA~\cite{FTC:COPPA:2013} regulations.
%, which is currently going unaddressed due to Apple's lack of regulation.

\dataSecurity
\paragraph{Data Security} While privacy labels provide a way for users to learn  what data is collected by an app and for what purpose, they do not indicate if the data is handled in a secure manner. Polisis can identify segments that address \textit{Data Security}, and further identify if segments that address \textit{Secure data storage} or \textit{Secure data transfer}. 
We further considered if apps indicate in their policies that they employ security practices while storing or transferring data and present our findings in \autoref{fig:security}. We find that only 26\% ($n=29,843$) and 33\% ($n=73,051$) of the apps that indicate in their privacy labels that they collect data that is used to track users and linked to users, respectively, also indicate in their privacy labels that they store or transfer data in a secure manner.

\paragraph{Changes to the Privacy Policy.} 
%The App Store does not provide a way for users to be notified of changes to an app's privacy label once the app has been downloaded. 
Apps may choose to notify users of updates to their privacy policies, and we found that 50\% ($n=273,865$) apps that we analyzed addressed the possibility of \textit{privacy-relevant} changes to their policies. However, 38\% ($n=103,070$) of these apps did not indicate a procedure in place to notify users of such changes, and 3\% ($9,173$) explicitly stated that users will receive \textit{no} notification of \textit{privacy-relevant} changes.

For example, the privacy policy from a developer, ChowNow~\cite{ChowNow:Policy}, which has over 3,000 apps in the Apple App Store, places the burden on users, asking that they periodically revisit the policy. The relevant snippet is shown below.

\begin{quote}
    \textit{We may update this Privacy Policy from time to time and without prior notice to you to reflect changes in our privacy practices. We will indicate at the top of this Privacy Policy when it was most recently updated, and we encourage you to revisit this page periodically to stay aware of any changes.}
\end{quote}

\paragraph{Do Not Track Policy.} While 113,921 apps that we analyzed state that they collect data that is used to track users, we identified only 13,183 of these apps that include a \textit{Do Not Track} statement in their privacy policy. Complicating matters, policies may state that they do not honor \textit{Do Not Track} requests from users. An example snippet from \textit{ChowNow}'s policy~\cite{ChowNow:Policy} is provided below.

\begin{quote}
    \textit{As discussed above, third parties such as advertising networks and analytics providers may collect information about your online activities over time and across different websites when you access or use the Services. Currently, various browsers offer a “Do Not Track” option, but there is no standard for commercial websites. At this time, we do not monitor, recognize, or honor any opt-out or do not track mechanisms, including general web browser “Do Not Track” settings and/or signals.}
\end{quote}

\paragraph{User Choice.} Privacy labels do not address choices that users have, leaving them with only the option whether they install the app at all or not. Apps may, however, highlight user choices within their policies. We found that 65\% ($n=360,011$) of the apps that we analyzed addressed user choices over the app's data collection practices. However, 33\% ($n=117,072$) of these apps left users with the only choice of \textit{not} using the service.
